# Supplementary material for: Validated Intent Compilation for Constrained Routing in LEO Mega-Constellations
Source: arXiv:2604.07264 source file (2026-04-08)
Supplement: Supplementary file 1 [file paper_appendix_reproducibility.tex]

% Reproducibility Appendix
% For inclusion as paper Appendix A

\section*{Appendix A: Reproducibility Details}
\label{sec:appendix_reproducibility}

This appendix documents the exact prompts, benchmark composition,
evaluation rubric, and verifier audit methodology used in our experiments,
enabling full reproduction of reported results.

\subsection*{A.1 LLM Compiler Configuration}

\begin{itemize}
\item \textbf{Model}: Qwen3.5-9B (GGUF quantization, served via LM Studio)
\item \textbf{Inference}: Local GPU (RTX 4060 8GB), OpenAI-compatible API
\item \textbf{Temperature}: 0.1
\item \textbf{Max tokens}: 2048
\item \textbf{Max repair retries}: 3
\item \textbf{Timeout}: 120s per API call
\end{itemize}

\subsection*{A.2 System Prompt}

The system prompt provides the constellation specification (20 planes
$\times$ 20 satellites = 400 nodes), the complete ConstraintProgram JSON
schema, all valid enum values (10 hard constraint types, 5 soft constraint
types, 14 regions, 8 traffic classes, 6 event types), target format
conventions, priority guidelines, and 6 compilation rules. The full
prompt is 101 lines (approximately 800 tokens) and is included in the
released codebase at \texttt{intent/compiler.py}.

\subsection*{A.3 Few-Shot Examples}

The compiler uses 6 in-context examples (3 user/assistant pairs)
covering the following intent categories:

\begin{table}[h]
\centering
\small
\begin{tabular}{clll}
\toprule
\textbf{\#} & \textbf{Intent Pattern} & \textbf{Constraint Types} & \textbf{Category} \\
\midrule
1 & Disable single node & \texttt{disable\_node} & Single \\
2 & Latency SLA on flow & \texttt{max\_latency\_ms} & Single \\
3 & Plane disable + polar + util & \texttt{disable\_plane}, \texttt{avoid\_lat}, \texttt{max\_util} & Compositional \\
4 & Event-triggered reroute & \texttt{reroute\_away}, \texttt{avoid\_lat} + condition & Conditional \\
5 & Flow SLA + region avoid & \texttt{max\_latency\_ms}, \texttt{avoid\_region} & Compositional \\
\bottomrule
\end{tabular}
\caption*{Few-shot examples span single, compositional, and conditional categories.
No infeasible examples are included, testing the model's zero-shot
infeasibility handling.}
\end{table}

\subsection*{A.4 Benchmark Composition}

The 240-intent benchmark is stratified across four categories:

\begin{table}[h]
\centering
\small
\begin{tabular}{lrl}
\toprule
\textbf{Category} & \textbf{N} & \textbf{Description} \\
\midrule
Single & 80 & One constraint type (disable, latency, avoid, etc.) \\
Compositional & 100 & 2--4 constraint types combined \\
Conditional & 30 & Event-triggered constraints (\texttt{if solar\_storm}, etc.) \\
Infeasible & 30 & Physically unrealizable (out-of-range nodes, impossible latency) \\
\bottomrule
\end{tabular}
\end{table}

\noindent Each benchmark entry contains: \texttt{id}, \texttt{category},
\texttt{intent\_text} (natural language), \texttt{constraint\_program}
(ground-truth JSON), \texttt{difficulty} (easy/medium/hard), and
\texttt{tags}. The benchmark is released at
\texttt{intent/benchmark/benchmark\_240.json}.

\subsection*{A.5 Evaluation Rubric}

Compiler output is scored against ground truth on four hierarchical
metrics, each requiring the previous to be true:

\begin{enumerate}
\item \textbf{Compiled}: The compiler produces a JSON that passes all
7 verifier checks (or, for infeasible intents, produces any parseable
JSON). Binary.

\item \textbf{Types Match}: All hard and soft constraint \texttt{type}
fields match the ground truth, compared as sorted multisets. Order-
insensitive.

\item \textbf{Targets Match}: All constraint \texttt{target} fields
match (e.g., \texttt{node:142}, \texttt{flow\_selector:0}). Requires
types match.

\item \textbf{Full Match (Values Match)}: All constraint \texttt{value}
fields match with numeric tolerance ($\epsilon = 10^{-6}$ relative).
String values are compared case-insensitively. This is the primary
accuracy metric reported in all tables.
\end{enumerate}

\noindent The \texttt{numeric\_eq} comparator uses
\texttt{math.isclose(a, b, rel\_tol=1e-6, abs\_tol=1e-6)} for numeric
values and case-insensitive string comparison for region/traffic names.
Constraint lists are compared order-insensitively (sorted by string
representation).

\subsection*{A.6 Ablation Configurations}

Four configurations are evaluated on the full 240-intent benchmark:

\begin{table}[h]
\centering
\small
\begin{tabular}{llll}
\toprule
\textbf{Config} & \textbf{Few-shot} & \textbf{Verifier} & \textbf{Repair Loop} \\
\midrule
Full pipeline & 6-shot & Yes & Up to 3 retries \\
No verifier & 6-shot & No & No \\
No repair & 6-shot & Yes & 1 attempt only \\
Zero-shot & 0-shot & Yes & Up to 3 retries \\
\bottomrule
\end{tabular}
\end{table}

\subsection*{A.7 Verifier Corruption Audit}

The verifier is tested on 8 corruption types $\times$ 30 injections
= 240 synthetic tests. Each corruption type targets a specific
verifier pass:

\begin{table}[h]
\centering
\small
\begin{tabular}{lll}
\toprule
\textbf{Corruption Type} & \textbf{Target Pass} & \textbf{Example} \\
\midrule
Missing \texttt{intent\_id} & Schema & Remove required field \\
Invalid priority & Schema & \texttt{priority: "urgent"} \\
Out-of-range node ID & Entity grounding & \texttt{node:454} in 400-node constellation \\
Invalid traffic class & Entity grounding & \texttt{traffic\_class: "gaming"} \\
Type mismatch & Type safety & \texttt{max\_latency\_ms} on \texttt{node:42} \\
Negative latency & Value range & \texttt{value: -50.0} \\
Latency below minimum & Physical admissibility & \texttt{value: 0.5} (min $\approx$ 2.5ms) \\
Invalid plane ID & Physical admissibility & \texttt{plane:25} in 20-plane constellation \\
\bottomrule
\end{tabular}
\end{table}

\noindent All 240 corrupted programs are correctly rejected (100\%
detection rate). Each of the 7 verifier passes catches at least one
corruption type, confirming non-overlapping coverage.

\subsection*{A.8 OOD Generalization Protocol}

Out-of-distribution evaluation uses 38 paraphrased intents (33 scorable
+ 5 deliberately ambiguous). Paraphrases are generated by varying:
vocabulary (``satellite'' $\to$ ``sat'', ``shut down'' $\to$ ``kill''),
sentence structure (imperative $\to$ declarative), specificity level
(explicit IDs $\to$ descriptive references), and combining constraint
patterns not seen in the 6-shot examples. Ambiguous intents (e.g.,
``optimize the network'') are scored qualitatively only.

\subsection*{A.9 End-to-End Routing Evaluation}

Constrained routing is evaluated across 4 scenarios $\times$ 3 random
seeds $\times$ 20 time steps. Each scenario applies compiled constraints
to the constellation topology, then routes 100 random OD pairs using
both GNN and Dijkstra routers. Metrics: packet delivery ratio (PDR)
and constraint violation count.

\subsection*{A.10 Code and Data Availability}

All code, benchmarks, trained models, and evaluation scripts are
released at: \texttt{github.com/LinkDry/Validated-Intent-Compilation-for-Constrained-Routing-in-LEO-Mega-Constellations}. The release includes:
\begin{itemize}
\item \texttt{intent/compiler.py}: LLM compiler with full prompt
\item \texttt{intent/verifier.py}: 8-pass deterministic validator with feasibility certification
\item \texttt{intent/benchmark/}: all benchmark JSON files
\item \texttt{scripts/eval\_*.py}: all evaluation scripts
\item \texttt{output/pretrain\_ctg3/best.pt}: trained GNN checkpoint
\item \texttt{output/*.json}: all raw experimental results
\end{itemize}
